# Supplementary material for: Transport map accelerated adaptive importance sampling, and application to inverse problems arising from multiscale stochastic reaction networks
Source: arXiv:1901.11269 source file (2020-07-27)
Supplement: Supplementary file 1 [file TETAIS_supplementary.pdf]

# MULTISCALE METHODS FOR STOCHASTIC CHEMICAL REACTION NETWORKS: SUPPLEMENTARY MATERIAL

SIMON L. COTTER\*, IOANNIS G. KEVREKIDIS†, AND PAUL RUSSELL‡

In this supplementary material, we discuss some recent advances in multiscale methods for stochastic reaction networks. Inverse problems arising in this area often lead to complex posterior distributions, which traditional MCMC methods can struggle to sample from.

We consider chemical reaction networks of  $N_s$  chemical species  $\{S_j\}_{j=1}^{N_s}$ , with population numbers given by  $X(t) = [X_1(t), X_2(t), \dots, X_{N_s}(t)]^\top \in \mathbb{N}_0^{N_s}$  reacting in a small reactor, through  $N_r$  different reaction channels. When population numbers of one or more of the chemical species in the reactor is small, as is the case with chemical reactions occurring within living cells, the sporadic and discrete way in which reactions occur can not be well modelled by deterministic continuous models, such as ODEs. In such a situation, we may wish to model the dynamics through a discrete stochastic model, such as a continuous time Markov chain.

For each reaction  $R_j$ , for  $j = 1, 2, \dots, N_r$ , there is a propensity or hazard function  $\alpha_j(X(t))$  which indicates how likely that reaction is to fire, defined by

$$\alpha_j(X(t)) = \lim_{dt \rightarrow 0} \mathbb{P}(\text{Reaction } R_j \text{ in the time interval } s \in [t, t + dt]).$$

If a system satisfies what is called *mass action kinetics*, then the form of the function  $\alpha_j$  is determined, up to a rate constant, by the reactants involved in that reaction:

$$\alpha_j(X) = k_j \prod_{m=1}^{N_s} \prod_{n=0}^{\nu_{j,m}-1} (X_m - n), \quad (\text{a.1})$$

where  $\nu_{j,m}$  is the  $m$ th component of the stoichiometric vector  $\nu_j$ ,  $X_m$  is the  $m$ th component of the state vector  $X$ , and the  $k_j$  are rate constants.

Following each reaction  $R_j$  there is an instantaneous change in the current state, as the reactants of the reaction are consumed, and the products produced. This is modelled by a change in the state vector  $X(t) = X(t) + \nu_j$  where  $\nu_j$  is that stoichiometric vector for reaction  $R_j$ .

The model can be represented as the following expression involving  $N_r$  different unit rate Poisson processes [4]  $Y_j$ , given by:

$$X(t) = X(0) + \sum_{j=1}^{N_r} \nu_j \int_0^t \alpha_j(X(s)) ds. \quad (\text{a.2})$$

---

\*School of Mathematics, University of Manchester, Manchester, UK. e: [simon.cotter@manchester.ac.uk](mailto:simon.cotter@manchester.ac.uk). SLC is grateful for EPSRC First grant award EP/L023393/1. SLC would like to thank the Isaac Newton Institute for Mathematical Sciences for support and hospitality during the programme ‘‘Uncertainty quantification for complex systems: theory and methodologies’’ when work on this paper was undertaken. This work was supported by: EPSRC grant number EP/K032208/1.

†Chemical and Biomolecular Engineering & Applied Mathematics and Statistics, Johns Hopkins University, Baltimore, MD 21218. The work of IGK was partially supported by the US National Science Foundation, by the US AFOSR, and by DARPA.

‡School of Mathematics, University of Manchester, Manchester, UK.

The master equation for this model is only solvable in certain situations, for example monomolecular networks [12], or for steady-state solutions for weakly reversible deficiency zero networks [2, 3]. Trajectories for this system can be sampled exactly, for instance using the Gillespie SSA [10], or its variants [1, 5, 11]. However, if the system is stiff, i.e. there are some reactions which are firing many times on a timescale for which others are unlikely to fire at all, then trajectories can become prohibitively expensive to simulate, since these methods simulate every single reaction event with the same cost. In such a system, one might employ multiscale methods in order to approximate trajectories at a lower cost than the exact algorithms.

One common approach is to invoke the quasi-equilibrium approximation QEA. This approximation makes the assumption that fast reactions enter quasi-equilibrium on a timescale which is negligible with respect to the timescale on which the slow dynamics in the system are evolving. This amounts to taking the asymptotic limit that the propensities of the “slow” reaction channels are equal to zero. This allows us to sample approximate trajectories of the slow reactions without the need to compute many fast reaction events.

This approach can work well when there is a large timescale gap between the fast and slow reactions in a system, but where the timescale gap is less pronounced, it can lead to significant errors [7]. Another approach is the constrained multiscale algorithm (CMA) [6, 8], based in part on the equation-free approach to multiscale computations [9, 13]. This approach also assumes quasi-equilibrium in the system, but takes into account the effect that the slow reactions can have on the invariant distribution of the fast variables in the system. For a more detailed description of this method, please refer to the literature [6].

Multiscale methods are not only of use when forward evaluations of the dynamics are costly, but can also be of use where we attempt to solve an inverse problem where the fast variables are unobservable. One approach in this situation would be to integrate over all possible trajectories of the fast variables, but this would almost always be prohibitively expensive. Another approach would be to use an appropriate multiscale approximation, so that the effective dynamics of the slow variables can be approximate without the need to consider the rapid fluctuations of the fast variables in the system.

**a.1. Likelihoods arising from stochastic reaction networks.** Suppose that we are able to exactly observe the number of molecules of each chemical species in a system which satisfies mass action kinetics, and which can be well approximated by (a.2). Suppose that we wish to be able to infer the value of the rate constants of each reaction from these observations. Even with no observational noise, since the dynamics of the system are stochastic, this still leads to a Bayesian inverse problem where we can only infer a joint probability distributions on the reaction parameters. Suppose that we are in state  $X(t) = X_0$ . There are two independent univariate random variables which decide when and what the next reaction in the system is. There is the  $j$ th waiting time  $\tau_j$  to the next reaction, which is given by an exponential random variable

$$\tau_j \sim \exp\left(\frac{1}{\alpha_0(X(t))}\right),$$

where  $\alpha_0(X(t)) = \sum_i^{N_r} \alpha_i(X(t))$  is the total propensity in the system. The second is a multinomial random variable  $r_j$  which dictates which reaction has occurred during

the  $j$ th reaction, which takes the value  $i \in \{1, 2, \dots, N_r\}$  with probability

$$\mathbb{P}(r_j = i) = \frac{\alpha_i(X(t))}{\alpha_0(X(t))}.$$

As such, in order to compute the likelihood of a particular trajectory given a possible realisation of the reaction parameters, it is sufficient to have access to the total time spent in each state, and the frequency of each reaction which led to leaving each state. From this formulation, we see that the random variables  $(\tau_j, r_j)$  only depend on the states  $\mathbf{X}(t_{j-1})$  and so are Markovian. This conditional independence means that we can group events together by what state the system was in when the event happened. We define two new random variables which depend on a state  $\mathbf{Y} \in \mathcal{S}$ , first the total time spent in state  $\mathbf{Y}$ ,

$$T(\mathbf{Y}) = \sum_{j=1}^M \tau_j \mathbf{I}(\mathbf{X}(t_{j-1}) = \mathbf{Y}).$$

This random variable,  $T(\mathbf{Y})$ , is a sum of exponentially distributed random variable, each with the rate  $\alpha_0(\mathbf{Y}; \mathbf{k})$ , and hence follows the Gamma distribution,

$$T(\mathbf{Y}) \sim \text{Gamma}(\alpha = K(\mathbf{Y}), \beta = \alpha_0(\mathbf{Y}; \mathbf{k})), \quad (\text{a.3})$$

where  $K(\mathbf{Y}) = \sum_{j=1}^M \mathbf{I}(\mathbf{X}(t_{j-1}) = \mathbf{Y})$ .

Similarly, we can define the reactions which occurred when the system was in state  $\mathbf{Y}$  as  $\mathbf{r}(\mathbf{Y}) = [r_1(\mathbf{Y}), \dots, r_{N_r}(\mathbf{Y})]^\top$  where

$$r_i(\mathbf{Y}) = \sum_{j=1}^M \mathbf{I}(r_j = i \text{ and } \mathbf{X}(t_{j-1}) = \mathbf{Y}).$$

Here all the random variables  $r_j$  follow the same multinomial distribution, and so

$$\mathbf{r}(\mathbf{Y}) \sim \text{Multinomial}(K(\mathbf{Y}), \mathbf{p}(\mathbf{Y})). \quad (\text{a.4})$$

The random variables defined in Equations (a.3) and (a.4) are sufficient statistics for the posterior distribution  $\pi(\mathbf{k}|D)$ . With these definitions we define two new structures

$$\mathbf{T} = [T(\mathbf{Y}_1), \dots, T(\mathbf{Y}_K)]^\top, \quad \text{and} \quad \mathbf{R} = [\mathbf{r}(\mathbf{Y}_1), \dots, \mathbf{r}(\mathbf{Y}_K)]^\top,$$

where  $K = |\mathcal{S}|$ , the number of states in  $\mathcal{S}$ , and each state  $\mathbf{Y}_i \in \mathcal{S}$  has been enumerated. We use these structures to define shorter notation,

$$\mathbf{T}_i = T(\mathbf{Y}_i), \quad \mathbf{R}_{ij} = r_j(\mathbf{Y}_i), \quad \text{and} \quad \mathbf{K}_i = K(\mathbf{Y}_i).$$

To construct the posterior distribution for the reaction rates,  $\mathbf{k}$ , in the chemical system, we formulate the likelihood using the sufficient statistics derived in the previous section. Due to the non-negativity of these reaction rates, we assign a Gamma prior distribution to each rate. Given the distributions in Equations (a.3) and (a.4) for our data, the likelihood of observing the data  $\mathbf{R}$  and  $\mathbf{T}$  is

$$\ell(\mathbf{R}, \mathbf{T}|\mathbf{k}) \propto \prod_{i=1}^K \text{Multi}(\mathbf{R}_i; \mathbf{K}_i, \mathbf{p}(\mathbf{Y}_i)) \text{Gamma}(\mathbf{T}_i; \mathbf{K}_i, \alpha_0(\mathbf{Y}_i)),$$

where again  $\mathbf{Y}_i \in \mathcal{S}$  and the propensities  $\alpha_i$  and probabilities  $p_i$  depend on the reaction rates  $\mathbf{k} = [k_1, k_2, \dots, k_{N_r}]^\top$  through the concept of mass action kinetics given in (a.1).

Our choice of Gamma prior distributions with hyper-parameters  $(a_i, b_i)$  results in the posterior distribution of the form

$$\begin{aligned} \pi(\mathbf{k}|\mathbf{R}, \mathbf{T}) &\propto \ell(\mathbf{R}, \mathbf{T}|\mathbf{k}) \prod_{i=1}^{N_r} \text{Gamma}(k_i; a_i, b_i) \\ &\propto \exp \left\{ \sum_{i=1}^K \left[ \mathbf{K}_i \log \alpha_0(\mathbf{Y}_i; \mathbf{k}) - \mathbf{T}_i \alpha_0(\mathbf{Y}_i; \mathbf{k}) + \sum_{j=1}^{N_r} \mathbf{R}_{ij} \log \mathbf{p}_j(\mathbf{Y}_i; \mathbf{k}) \right] \right. \\ &\quad \left. + \sum_{i=1}^{N_r} ((a_i - 1) \log k_i - b_i k_i) \right\}. \end{aligned} \quad (\text{a.5})$$

**a.2. Approximation of likelihoods in multiscale chemical networks.** Suppose now that we only observe the slower variables in a multiscale chemical system of this type. Suppose that  $n_r < N_r$  is the number of slow reactions in the system, and the slow reactions are given by  $\{R_{s_1}, R_{s_2}, \dots, R_{s_{n_r}}\} \subset \{R_1, R_2, \dots, R_{N_r}\}$ . The propensities of the slow reactions  $\alpha_{s_i}$  may depend on the value of the fast variables which is unknown. However, the invariant distribution of the fast variables conditioned on the slow variables in the system can be approximated using a multiscale method, such as the QEA or the CMA. Once the approximations have been made, we arrive at approximate *effective* propensities  $\bar{\alpha}_{s_i}$ , which have been averaged over the computed invariant distributions of the fast variables. Then the approximate effective dynamics on the slow variable  $S(t)$  are given by

$$S(t) = S(0) + \sum_{j=1}^{n_r} \nu_{s_j} \int_0^t \bar{\alpha}_{s_j}(S(s)) ds. \quad (\text{a.6})$$

In turn, the approximate posterior distribution on the reaction parameters  $\mathbf{k}$  is then given by

$$\begin{aligned} \pi(\mathbf{k}|\mathbf{R}, \mathbf{T}) &\propto \ell(\mathbf{R}, \mathbf{T}|\mathbf{k}) \prod_{i=1}^{n_r} \text{Gamma}(k_i; a_i, b_i) \\ &\propto \exp \left\{ \sum_{i=1}^K \left[ \mathbf{K}_i \log \bar{\alpha}_0(\mathbf{Y}_i; \mathbf{k}) - \mathbf{T}_i \bar{\alpha}_0(\mathbf{Y}_i; \mathbf{k}) + \sum_{j=1}^{n_r} \mathbf{R}_{ij} \log \bar{\mathbf{p}}_j(\mathbf{Y}_i; \mathbf{k}) \right] \right. \\ &\quad \left. + \sum_{i=1}^{n_r} ((a_i - 1) \log k_i - b_i k_i) \right\}, \end{aligned} \quad (\text{a.7})$$

where  $\bar{\alpha}_0(\mathbf{Y}_i; \mathbf{k}) = \sum_{j=1}^{n_r} \bar{\alpha}_j(\mathbf{Y}_i; \mathbf{k})$  is the total of the effective propensities,  $n_r$  is the number of slow reactions,  $\bar{\mathbf{p}}(\mathbf{Y}_i; \mathbf{k})$  is the multiscale approximation of the expected proportion of each slow reaction at state  $\mathbf{Y}_i$  and with reaction rates  $\mathbf{k}$  and the data is limited only to changes in the slow variable due to the occurrence of slow reactions.

## REFERENCES

- [1] D. ANDERSON, *A modified next reaction method for simulating chemical systems with time dependent propensities and delays*, The Journal of chemical physics, 127 (2007), p. 214107.
- [2] D. ANDERSON AND S. COTTER, *Product-form stationary distributions for deficiency zero networks with non-mass action kinetics*, Bulletin of mathematical biology, 78 (2016), pp. 2390–2407.
- [3] D. ANDERSON, G. CRACIUN, AND T. KURTZ, *Product-form stationary distributions for deficiency zero chemical reaction networks*, Bulletin of mathematical biology, 72 (2010), pp. 1947–1970.
- [4] D. ANDERSON AND T. KURTZ, *Continuous time markov chain models for chemical reaction networks*, in Design and analysis of biomolecular circuits, Springer, 2011, pp. 3–42.
- [5] Y. CAO, H. LI, AND L. PETZOLD, *Efficient formulation of the stochastic simulation algorithm for chemically reacting systems*, The journal of chemical physics, 121 (2004), pp. 4059–4067.
- [6] S. COTTER, *Constrained approximation of effective generators for multiscale stochastic reaction networks and application to conditioned path sampling*, Journal of Computational Physics, 323 (2016), pp. 265–282.
- [7] S. COTTER AND R. ERBAN, *Error analysis of diffusion approximation methods for multiscale systems in reaction kinetics*, SIAM Journal on Scientific Computing, 38 (2016), pp. B144–B163.
- [8] S. COTTER, K. ZYGALAKIS, I. KEVREKIDIS, AND R. ERBAN, *A constrained approach to multiscale stochastic simulation of chemically reacting systems*, The Journal of Chemical Physics, 135 (2011), p. 094102.
- [9] R. ERBAN, I. KEVREKIDIS, D. ADALSTEINSSON, AND T. ELSTON, *Gene regulatory networks: A coarse-grained, equation-free approach to multiscale computation*, The Journal of chemical physics, 124 (2006), p. 084106.
- [10] D. GILLESPIE, *Exact stochastic simulation of coupled chemical reactions*, The Journal of Physical Chemistry, 81 (1977), pp. 2340–2361.
- [11] ———, *Stochastic simulation of chemical kinetics*, Annu. Rev. Phys. Chem., 58 (2007), pp. 35–55.
- [12] T. JAHNKE AND W. HUISINGA, *Solving the chemical master equation for monomolecular reaction systems analytically*, Journal of Mathematical Biology, 54 (2007), pp. 1–26.
- [13] I. KEVREKIDIS, C.W. GEAR, J. HYMAN, P. KEVREKIDIS, O. RUNBORG, C. THEODOROPOULOS, ET AL., *Equation-free, coarse-grained multiscale computation: Enabling microscopic simulators to perform system-level analysis*, Communications in Mathematical Sciences, 1 (2003), pp. 715–762.
